# Supplementary material for: SPARQ-SGD: Event-Triggered and Compressed Communication in Decentralized Stochastic Optimization
Source: arXiv:1910.14280 source file (2020-02-24)
Supplement: Supplementary file 1 [file suppl_dec_sgd.tex]

We restate the sequence of updates for Algorithm \ref{alg_dec_sgd} in matrix form for reference (see Remark \ref{mat_not}):
\begin{align*}
X^{(t+\frac{1}{2})} & = X^{(t)} - \eta_t \partial F(X^{(t)},\xi^{(t)}) \\
\hat{X}^{(t+1)} & = \hat{X}^{{(t)}} + Q((X^{{(t+\frac{1}{2})}} - \hat{X}^{{(t)}})P^{(t)} ) \\
X^{{(t+1)}} & = X^{{(t+\frac{1}{2})}} + \gamma\hat{X}^{{(t+1)}}(W-I) 
\end{align*}
$P^{(t)} \in \mathbb{R}^{n \times n} $ is a diagonal matrix with entry $1$ for nodes that communicate in time step $t$ with regard to the triggering condition and entry 0 for nodes which don't. \\
These equalities are used throughout the proofs in this section. % \\ \\ 
%We first note the following Lemma which is useful in proofs for Theorem \ref{thm_cvx}, Theorem \ref{thm_noncvx_var} and Theorem \ref{thm_noncvx_fix}
%------------Lemma-------
\subsection{Proof of Lemma \ref{lem_dec_sgd}} \label{proof_lem_dec_sgd}
\begin{lemma*} (Restating Lemma \ref{lem_dec_sgd} )
	Consider the sequence of updates as in Algorithm \ref{alg_dec_sgd} with $\eta_t = \frac{b}{a+t } $ (where $a \geq \frac{5}{p}, \, b > 0$) as the learning rate.
%	\begin{align*}
%	X^{(t+\frac{1}{2})} = X^{(t)} - \eta_t \partial F(X^{(t)},\xi^{(t)}) \\
%	\hat{X}^{(t+1)} = \hat{X}^{{(t)}} + Q((X^{{(t+\frac{1}{2})}} - \hat{X}^{{(t)}})P^{(t)} ) \\
%	X^{{(t+1)}} = X^{{(t+\frac{1}{2})}} + \gamma\hat{X}^{{(t+1)}}(W-I) 
%	\end{align*}
%	where $P^{(t)}$ is a diagonal matrix with entry $1$ for nodes that communicate in time step $t$ with regard to the triggering condition.
	Then we have:
	\begin{align*}
	\mathbb{E}\sum_{j=1}^n \Vert \bar{x}_{t} - x_t^{(j)} \Vert^2 = \mathbb{E}\Vert\Bar{X}^{{(t)}} - X^{{(t)}}\Vert_F^2 \leq \frac{20A\eta_{{t}}^2}{p^2}
	\end{align*}
	where $p = \frac{\delta^2 \omega}{644} $, $\delta := 1 - | \lambda_2(W)|$, $\omega$ is contraction parameter for quantization operator $Q$ and  $A=2nG^2 + \frac{p}{2} \left(\frac{8nG^2}{\omega} + \frac{5\omega n c_0}{4} \right) $
\end{lemma*}
\begin{proof}
	Consider the expression 
	\begin{align} \label{suppl_et_eqn}
		e_{t+1} := \Vert X^{(t+1)} - \Bar{X}^{(t+1)} \Vert_F^2 + \Vert X^{(t+1)} - \hat{X}^{(t+2)} \Vert_F^2
	\end{align}
	The first term of (\ref{suppl_et_eqn}) can be bounded as:
	\begin{align*}
	\Vert X^{(t+1)} - \Bar{X}^{(t+1)} \Vert_F^2 & = \Vert X^{(t+\frac{1}{2})} - \Bar{X}^{(t+1)} + \gamma \hat{X}^{(t+1)} (W-I)  \Vert_F^2 \\
%	\intertext{Using the fact that $\Bar{X}^{(t+1)} = \Bar{X}^{(t+\frac{1}{2})}$ (see Remark 3):}
	& \stackrel{(\ref{mean_seq_iter})}{=} \Vert X^{(t+\frac{1}{2})} - \Bar{X}^{(t+\frac{1}{2})} + \gamma \hat{X}^{(t+1)} (W-I)  \Vert_F^2 \\
	& = \Vert X^{(t+\frac{1}{2})} - \Bar{X}^{(t+\frac{1}{2})} + \gamma ({X}^{(t+\frac{1}{2})} - \Bar{X}^{(t+\frac{1}{2})}) (W-I) + \gamma (\hat{X}^{(t+1)}-X^{(t+\frac{1}{2})}) (W-I)  \Vert_F^2 \\
	& = \Vert (X^{(t+\frac{1}{2})} - \Bar{X}^{(t+\frac{1}{2})})((1-\gamma)I + \gamma W) + \gamma (\hat{X}^{(t+1)}-X^{(t+\frac{1}{2})}) (W-I)  \Vert_F^2 \\
%	\intertext{Using the fact $\Vert A + B \Vert_F^2 \leq (1+\alpha)\Vert A\Vert_F^2 + (1+\alpha^{-1})\Vert B \Vert_F^2$ for any $\alpha >0$, }
	& \stackrel{(\ref{bound_l2_sum})}{\leq} (1+\alpha_1)\Vert (X^{(t+\frac{1}{2})} - \Bar{X}^{(t+\frac{1}{2})})((1-\gamma)I + \gamma W)\Vert_F^2 + (1+\alpha_1^{-1}) \Vert \gamma (\hat{X}^{(t+1)}-X^{(t+\frac{1}{2})}) (W-I)  \Vert_F^2 \\
%	\intertext{Using the fact that for any $A \in \mathbb{R}^{d \times n},B \in \mathbb{R}^{n \times n}$, $\Vert AB \Vert_F \leq \Vert A \Vert_F \Vert B\Vert_2$, }
	& \stackrel{(\ref{bound_frob_mult})}{\leq} (1+\alpha_1)\Vert (X^{(t+\frac{1}{2})} - \Bar{X}^{(t+\frac{1}{2})})((1-\gamma)I + \gamma W)\Vert_F^2 + (1+\alpha_1^{-1}) \gamma^2 \Vert  (\hat{X}^{(t+1)}-X^{(t+\frac{1}{2})})\Vert_F^2 .\Vert(W-I) \Vert_2^2 
	\end{align*}
	The first term can be bounded as:
	\begin{align*}
	\Vert (X^{(t+\frac{1}{2})} - \Bar{X}^{(t+\frac{1}{2})})((1-\gamma)I + \gamma W)\Vert_F & \leq (1-\gamma)\Vert X^{(t+\frac{1}{2})} - \Bar{X}^{(t+\frac{1}{2})} \Vert_F + \gamma \Vert (X^{(t+\frac{1}{2})} - \Bar{X}^{(t+\frac{1}{2})} )W\Vert_F \\ 
%	\intertext{Using the definition for $\bar{X}^{(t+\frac{1}{2})} = X^{(t+\frac{1}{2})}\frac{\mathbbm{1}\mathbbm{1}^T}{n} $}
	& \stackrel{(\ref{mean_prop})}{=} (1-\gamma)\Vert X^{(t+\frac{1}{2})} - \Bar{X}^{(t+\frac{1}{2})} \Vert_F + \gamma \left\Vert (X^{(t+\frac{1}{2})} - \Bar{X}^{(t+\frac{1}{2})})\left (W - \frac{\mathbbm{1}\mathbbm{1}^T}{n} \right) \right\Vert_F \\
%	\intertext{Using remark 4,}
	& \stackrel{(\ref{bound_frob_mult}),(\ref{bound_W_mat})}{\leq} (1-\gamma) \Vert X^{(t+\frac{1}{2})} - \Bar{X}^{(t+\frac{1}{2})} \Vert_F + \gamma \Vert X^{(t+\frac{1}{2})} - \Bar{X}^{(t+\frac{1}{2})} \Vert_F (1-\delta) \\
	& =(1-\gamma \delta) \Vert X^{(t+\frac{1}{2})} - \Bar{X}^{(t+\frac{1}{2})} \Vert_F
	\end{align*}
	Substituting above and using $\beta = \text{max}_i \{ 1- \lambda_i(W) \} \Rightarrow \Vert W-I \Vert_2^2 \leq \beta^2 $, we get:
	\begin{align*}
	\Vert X^{(t+1)} - \Bar{X}^{(t+1)} \Vert_F^2 \leq (1+\alpha_1)(1-\gamma \delta)^2 \Vert X^{(t+\frac{1}{2})} - \Bar{X}^{(t+\frac{1}{2})} \Vert_F^2 + (1+\alpha_1^{-1}) \gamma^2 \beta^2  \Vert  {X}^{(t+\frac{1}{2})}-\hat{X}^{(t+1)}\Vert_F^2
	\end{align*}
	Taking expectation w.r.t the entire process, we get:
	\begin{align} \label{suppl_et_eqn_t1}
	\mathbb{E} \Vert X^{(t+1)} - \Bar{X}^{(t+1)} \Vert_F^2 \leq (1+\alpha_1)(1-\gamma \delta)^2 \mathbb{E} \Vert X^{(t+\frac{1}{2})} - \Bar{X}^{(t+\frac{1}{2})} \Vert_F^2 + (1+\alpha_1^{-1}) \gamma^2 \beta^2 \mathbb{E} \Vert  {X}^{(t+\frac{1}{2})}-\hat{X}^{(t+1)}\Vert_F^2
	\end{align}
	Consider the second term in (\ref{suppl_et_eqn}) and take expectation w.r.t entire process:
	\begin{align*}
	\mathbb{E} \Vert X^{(t+1)} - \hat{X}^{(t+2)}\Vert_F^2 & = \mathbb{E} \Vert X^{(t+1)} - \hat{X}^{(t+1)} - Q ( (X^{(t+\frac{3}{2})} - \hat{X}^{(t+1)}) P^{(t+1)} )\Vert_F^2 \\
	& = \mathbb{E} \Vert X^{(t+\frac{3}{2})} - \hat{X}^{(t+1)}+ X^{(t+1)} - X^{(t+\frac{3}{2})} - Q ( (X^{(t+\frac{3}{2})} - \hat{X}^{(t+1)}) P^{(t+1)} )\Vert_F^2 \\
%	\intertext{For any constant $\alpha_2 > 0$,}
	& \stackrel{(\ref{bound_l2_sum})}{\leq}  (1+\alpha_2) \mathbb{E} \Vert X^{(t+\frac{3}{2})} - \hat{X}^{(t+1)} - Q ( (X^{(t+\frac{3}{2})} - \hat{X}^{(t+1)}) P^{(t+1)} )\Vert_F^2 + (1+\alpha_2^{-1})\mathbb{E}\Vert X^{(t+1)} - X^{(t+\frac{3}{2})} \Vert_F^2 \\
	& = (1+\alpha_2) \mathbb{E} \Vert X^{(t+\frac{3}{2})} - \hat{X}^{(t+1)} - Q ( (X^{(t+\frac{3}{2})} - \hat{X}^{(t+1)}) P^{(t+1)} )\Vert_F^2 + (1+\alpha_2^{-1})\mathbb{E}\Vert \eta_{t+1} \partial F (X^{(t+1)}, \xi^{(t+1)}) \Vert_F^2 \\
	& \stackrel{ (\ref{bound_grad})}{\leq} (1+\alpha_2) \mathbb{E} \Vert X^{(t+\frac{3}{2})} - \hat{X}^{(t+1)} - Q ( (X^{(t+\frac{3}{2})} - \hat{X}^{(t+1)}) P^{(t+1)} )\Vert_F^2 + (1+\alpha_2^{-1}) \eta_{t+1}^2nG^2 \\
	& = (1+\alpha_2)  \mathbb{E} \Vert (X^{(t+\frac{3}{2})} - \hat{X}^{(t+1)})P^{(t+1)} - Q ( (X^{(t+\frac{3}{2})} - \hat{X}^{(t+1)}) P^{(t+1)} )\Vert_F^2  \\
	&  \hspace{2cm} + (1+\alpha_2) \mathbb{E} \Vert (X^{(t+\frac{3}{2})} - \hat{X}^{(t+1)})(I - P^{(t+1)})\Vert_F^2  + (1+\alpha_2^{-1}) \eta_{t+1}^2nG^2 \\
%	\intertext{Using the compression property of operator $Q$, }
	& \stackrel{(\ref{bound_comp})}{\leq} (1+\alpha_2) \mathbb{E} \left[(1-\omega) \Vert (X^{(t+\frac{3}{2})} - \hat{X}^{(t+1)})P^{(t+1)} \Vert_F^2 +  \Vert (X^{(t+\frac{3}{2})} - \hat{X}^{(t+1)})(I - P^{(t+1)})\Vert_F^2 \right] \\
	& \hspace{2cm} + (1+\alpha_2^{-1}) \eta_{t+1}^2nG^2  
	\intertext{Adding and subtracting $ (1+\alpha_2)(1-\omega) \mathbb{E} \Vert (X^{(t+\frac{3}{2})} - \hat{X}^{(t+1)})(I - P^{(t+1)})\Vert_F^2$,}
	& = (1+\alpha_2) \mathbb{E} \left[ (1-\omega)  \Vert X^{(t+\frac{3}{2})} - \hat{X}^{(t+1)} \Vert_F^2 + \omega  \Vert (X^{(t+\frac{3}{2})} - \hat{X}^{(t+1)})(I - P^{(t+1)})\Vert_F^2 \right] + (1+\alpha_2^{-1}) \eta_{t+1}^2nG^2 \\
%	\end{align*}
%	The second term in above expresison (multiplied by $(I - P^{(t+1)})$ ) denotes the norm of nodes which did not communicate in timestep $(t+1)$ and thus should be bounded by the triggering condition:
%	\begin{align}
	& \stackrel{(\ref{bound_trig})}{\leq} (1+\alpha_2) (1-\omega) \mathbb{E} \Vert X^{(t+\frac{3}{2})} - \hat{X}^{(t+1)} \Vert_F^2 +(1+\alpha_2)\omega n c_0 \eta_{t+1}^2  + (1+\alpha_2^{-1}) \eta_{t+1}^2nG^2  \\
	& = (1+\alpha_2) (1-\omega) \mathbb{E} \Vert X^{(t+1)}  - \eta_{t+1} \partial F(X^{(t+1)},\xi^{(t+1)}) -  \hat{X}^{(t+1)} \Vert_F^2 + (1+\alpha_2)\omega n c_0 \eta_{t+1}^2 \\
	& \hspace{2cm} + (1+\alpha_2^{-1}) \eta_{t+1}^2nG^2 \\
%	\intertext{For any constant $\alpha_3 > 0$, we have:}
	& \stackrel{(\ref{bound_l2_sum})}{\leq} (1+\alpha_3) (1+\alpha_2) (1-\omega) \mathbb{E} \Vert X^{(t+1)}  -  \hat{X}^{(t+1)} \Vert_F^2 +  (1+\alpha_3^{-1}) (1+\alpha_2) (1-\omega) \mathbb{E} \Vert \eta_{t+1} \partial F(X^{(t+1)},\xi^{(t+1)}) \Vert_F^2 \\
	& \hspace{2cm}+ (1+\alpha_2)\omega n c_0 \eta_{t+1}^2 + (1+\alpha_2^{-1}) \eta_{t+1}^2nG^2 \\
	& \stackrel{( \ref{bound_grad})}{\leq} (1+\alpha_3) (1+\alpha_2) (1-\omega) \mathbb{E} \Vert X^{(t+1)}  -  \hat{X}^{(t+1)} \Vert_F^2 +  (1+\alpha_3^{-1}) (1+\alpha_2) (1-\omega) \eta_{t+1}^2 nG^2 \\
	& \hspace{2cm}+ (1+\alpha_2)\omega n c_0 \eta_{t+1}^2 + (1+\alpha_2^{-1}) \eta_{t+1}^2nG^2 \\
	& = (1+\alpha_3) (1+\alpha_2) (1-\omega) \mathbb{E} \Vert X^{(t+\frac{1}{2})} + \gamma \hat{X}^{(t+1)} (W-I)  -  \hat{X}^{(t+1)} \Vert_F^2 +  (1+\alpha_3^{-1}) (1+\alpha_2) (1-\omega) \eta_{t+1}^2 nG^2 \\
	& \hspace{2cm} + (1+\alpha_2)\omega n c_0 \eta_{t+1}^2 + (1+\alpha_2^{-1}) \eta_{t+1}^2nG^2 \\
%	\intertext{Using Remark 3 (specifically,  $\Bar{X}^{(t+\frac{1}{2})}(W-I) = 0$),}
	& \stackrel{(\ref{mean_prop})}{=} (1+\alpha_3) (1+\alpha_2) (1-\omega)\mathbb{E} \Vert (X^{(t+\frac{1}{2})} - \hat{X}^{(t+1)})((1+\gamma)I - \gamma W) + \gamma (X^{(t+\frac{1}{2})}- \Bar{X}^{(t+\frac{1}{2})})(W-I) \Vert_F^2 \\
	& \hspace{2cm} +  (1+\alpha_3^{-1}) (1+\alpha_2) (1-\omega) \eta_{t+1}^2 nG^2 + (1+\alpha_2)\omega n c_0 \eta_{t+1}^2 + (1+\alpha_2^{-1}) \eta_{t+1}^2nG^2 \\
%	\intertext{For any $\alpha_4 > 0 $, we have:}
	&\stackrel{(\ref{bound_l2_sum})}{ \leq} (1+\alpha_4) (1+\alpha_3) (1+\alpha_2) (1-\omega) \mathbb{E} \Vert (X^{(t+\frac{1}{2})} - \hat{X}^{(t+1)})((1+\gamma)I - \gamma W) \Vert_F^2 \\
	& \hspace{1cm} + (1+\alpha_4^{-1}) (1+\alpha_3) (1+\alpha_2) (1-\omega) \mathbb{E} \Vert \gamma (X^{(t+\frac{1}{2})}- \Bar{X}^{(t+\frac{1}{2})})(W-I) \Vert_F^2 \\
	& \hspace{2cm} +  (1+\alpha_3^{-1}) (1+\alpha_2) (1-\omega) \eta_{t+1}^2 nG^2 + (1+\alpha_2)\omega n c_0 \eta_{t+1}^2 + (1+\alpha_2^{-1}) \eta_{t+1}^2nG^2 
	\end{align*}
	Using $\Vert (1+\gamma)I - \gamma W \Vert_2 = \Vert I + \gamma (I - W) \Vert_2 = 1 +  \gamma \Vert I-W \Vert_2  = 1 + \gamma \beta $ (by definition of $\beta = \text{max}_i \{ 1- \lambda_i(W) \}$) and (\ref{bound_frob_mult}):
	\begin{align} \label{suppl_et_eqn_t2}
	& \leq (1+\gamma \beta )^2 (1+\alpha_4) (1+\alpha_3) (1+\alpha_2) (1-\omega)\mathbb{E} \Vert X^{(t+\frac{1}{2})} - \hat{X}^{(t+1)}\Vert_F^2 \notag \\
	& \hspace{1cm} + \gamma^2 \beta^2 (1+\alpha_4^{-1}) (1+\alpha_3) (1+\alpha_2) (1-\omega) \mathbb{E} \Vert X^{(t+\frac{1}{2})}- \Bar{X}^{(t+\frac{1}{2})} \Vert_F^2 \notag \\
	& \hspace{1cm} +  (1+\alpha_3^{-1}) (1+\alpha_2) (1-\omega) \eta_{t+1}^2 nG^2 + (1+\alpha_2)\omega n c_0 \eta_{t+1}^2 + (1+\alpha_2^{-1}) \eta_{t+1}^2nG^2 
	\end{align}
	Thus combining the bounds for the first (\ref{suppl_et_eqn_t1}) and second (\ref{suppl_et_eqn_t2}) term of $\mathbb{E}[e_{t+1}]$ , we get:
	\begin{align} \label{suppl_et_eqn_total}
	\mathbb{E} [e_{t+1}] & = \mathbb{E} \Vert X^{(t+1)} - \Bar{X} \Vert_F^2 + \mathbb{E} \Vert X^{(t+1)} - \hat{X}^{(t+2)} \Vert_F^2  \notag \\ 
	& \leq (1+\alpha_1)(1-\gamma \delta)^2 \mathbb{E}\Vert X^{(t+\frac{1}{2})} - \Bar{X}^{(t+\frac{1}{2})} \Vert_F^2 + (1+\alpha_1^{-1}) \gamma^2 \beta^2 \mathbb{E} \Vert  {X}^{(t+\frac{1}{2})}-\hat{X}^{(t+1)}\Vert_F^2 \notag \\ 
	& \hspace{0.5cm} + (1+\gamma \beta )^2 (1+\alpha_4) (1+\alpha_3) (1+\alpha_2) (1-\omega) \mathbb{E} \Vert X^{(t+\frac{1}{2})} - \hat{X}^{(t+1)}\Vert_F^2  \notag \\
	& \hspace{0.5cm} + \gamma^2 \beta^2 (1+\alpha_4^{-1}) (1+\alpha_3) (1+\alpha_2) (1-\omega) \mathbb{E} \Vert X^{(t+\frac{1}{2})}- \Bar{X}^{(t+\frac{1}{2})} \Vert_F^2 +  (1+\alpha_3^{-1}) (1+\alpha_2) (1-\omega) \eta_{t+1}^2 nG^2  \notag \\
	& \hspace{0.5cm}+ (1+\alpha_2)\omega n c_0 \eta_{t+1}^2 + (1+\alpha_2^{-1}) \eta_{t+1}^2nG^2
	\end{align}
	Define the following:
	\begin{align*}
	\pi_1 (\gamma) & := \gamma^2 \beta^2 (1+\alpha_1^{-1}) + (1+\gamma \beta )^2 (1+\alpha_4) (1+\alpha_3) (1+\alpha_2) (1-\omega) \\
	\pi_2 (\gamma) & := (1-\delta \gamma)^2(1+\alpha_1) + \gamma^2 \beta^2 (1+\alpha_4^{-1}) (1+\alpha_3) (1+\alpha_2) (1-\omega) \\
	\pi_3 & := (1+\alpha_3^{-1}) (1+\alpha_2) (1-\omega) nG^2 + (1+\alpha_2)\omega n c_0 + (1+\alpha_2^{-1})nG^2 
	\end{align*}
	Thus the above bound on $\mathbb{E}[e_{t+1}]$ in (\ref{suppl_et_eqn_total}) can be rewritten as:
	\begin{align*}
	\mathbb{E} [e_{t+1}] & \leq \pi_1 (\gamma) \mathbb{E} \Vert {X}^{(t+\frac{1}{2})} - \hat{X}^{(t+1)} \Vert_F^2 + \pi_2 (\gamma) \mathbb{E} \Vert X^{(t+\frac{1}{2})} - \Bar{X}^{(t+\frac{1}{2})} \Vert_F^2 + \pi_3 \eta_{t+1}^2 \\
	& \leq max \{ \pi_1 (\gamma) , \pi_2 (\gamma) \} \, \mathbb{E} \left[ \Vert {X}^{(t+\frac{1}{2})} - \hat{X}^{(t+1)} \Vert_F^2 + \Vert X^{(t+\frac{1}{2})} - \Bar{X}^{(t+\frac{1}{2})} \Vert_F^2 \right] + \pi_3 \eta_{t+1}^2
	\end{align*}
	Calculation of $ max \{ \pi_1 (\gamma) , \pi_2 (\gamma) \}$ and $\pi_3$ is given in Lemma \ref{suppl_lem_coeff_calc}. This yields:
	\begin{align*}
	\mathbb{E}[e_{t+1}] \leq \left( 1 - \frac{\delta^2 \omega}{644} \right) \mathbb{E}  \left[ \Vert {X}^{(t+\frac{1}{2})} - \hat{X}^{(t+1)} \Vert_F^2 + \Vert X^{(t+\frac{1}{2})} - \Bar{X}^{(t+\frac{1}{2})} \Vert_F^2 \right] + \left( \frac{8nG^2}{\omega} + \frac{5\omega n c_0}{4} \right) \eta_t^2
	\end{align*}
	where we've used the fact that $\eta_t \geq \eta_{t+1}$ \\
	Defining $p := \frac{\delta^2\omega}{644}$, $c_1:= \left( \frac{8nG^2}{\omega} + \frac{5\omega n c_0}{4} \right) $ and using defintion of $e_{t+1} =  \left[ \Vert X^{{(t+1)}} - \Bar{X}^{{(t+1)}} \Vert_F^2 + \Vert X^{{(t+1)}} - \hat{X}^{{(t+2)}} \Vert_F^2 \right] $, 
	\begin{align*}
	\mathbb{E} \left[ \Vert X^{{(t+1)}} - \Bar{X}^{{(t+1)}} \Vert_F^2 + \Vert X^{{(t+1)}} - \hat{X}^{{(t+2)}} \Vert_F^2 \right] & \leq (1-p)( \mathbb{E} \Vert X^{{(t+\frac{1}{2})}} - \Bar{X}^{{(t+\frac{1}{2})}} \Vert_F^2 + \mathbb{E}\Vert X^{{(t+\frac{1}{2})}} - \hat{X}^{{(t+1)}} \Vert_F^2 ) + c_1 \eta_t^2
	\end{align*}
	Using the fact that $\Bar{X}^{{(t+\frac{1}{2})}} = \Bar{X}^{{(t)}} - \eta_{t}\partial F(X^{(t)}, \xi^{(t)} )   \frac{\mathbbm{1}\mathbbm{1}^T}{n}  $:
	\begin{align*}
	& = (1-p)\mathbb{E}\left\Vert \Bar{X}^{{(t)}} - X^{{(t)}} -  \eta_{t}\partial F(X^{(t)}, \xi^{(t)} )\left(   \frac{\mathbbm{1}\mathbbm{1}^T}{n} - I \right) \right\Vert_F^2 + (1-p)\mathbb{E}\left\Vert \hat{X}^{{(t+1)}} - X^{{(t)}} + \eta_{t} \partial F(X^{(t)}, \xi^{(t)} )\right\Vert_F^2 + c_1 \eta_t^2 \\
	& \stackrel{(\ref{bound_l2_sum})}{\leq} (1-p)(1+\alpha_1^{-1})\mathbb{E}\left[ \Vert\Bar{X}^{{(t)}} - X^{{(t)}}\Vert_F^2  + \Vert \hat{X}^{{(t+1)}} - X^{{(t)}} \Vert_F^2 \right] + (1-p)(1+\alpha_1) \mathbb{E}\left\Vert \eta_{t}\partial F(X^{(t)}, \xi^{(t)} )\left(   \frac{\mathbbm{1}\mathbbm{1}^T}{n} - I \right) \right\Vert_F^2  \\
	& \hspace{1cm} + (1-p)(1+\alpha_1) \mathbb{E}\left\Vert \eta_{t}\partial F(X^{(t)}, \xi^{(t)} )\right\Vert_F^2 + c_1 \eta_t^2 \\
%	\intertext{Using $\mathbb{E} \left\Vert \eta_{t}\partial F(X^{(t)}, \xi^{(t)} )\right\Vert_F^2  \leq \eta_{{t}} nG^2 $ and $\Vert \frac{\mathbbm{1}\mathbbm{1}^T}{n} - I \Vert_2^2 = 1 $ }
	& \stackrel{(\ref{bound_grad}),(\ref{bound_W_mat})}{\leq} (1-p) (1+\alpha_1^{-1})\mathbb{E}\left[ \Vert\Bar{X}^{{(t)}} - X^{{(t)}}\Vert_F^2  + \Vert \hat{X}^{{(t+1)}} - X^{{(t)}} \Vert_F^2 \right]  + (1-p)(1+\alpha_1) 2G^2n \eta_{t}^2 + c_1 \eta_t^2 \\
%	\intertext{Setting $\alpha_1 = \frac{2}{p}$, we have: }
	&\stackrel{ ( \alpha_1 = \frac{2}{p} ) }{\leq} \left( 1-\frac{p}{2} \right)\mathbb{E}\left[ \Vert\Bar{X}^{{(t)}} - X^{{(t)}}\Vert_F^2  + \Vert \hat{X}^{{(t+1)}} - X^{{(t)}} \Vert_F^2 \right] + \frac{4n}{p}\eta_{t}^2G^2 + c_1 \eta_t^2
	\end{align*}
	Define $A := 2nG^2 + \frac{p c_1}{2}$ (where $c_1= \left( \frac{8nG^2}{\omega} + \frac{5\omega n c_0}{4} \right) $ as above), thus we have the following relation:
	\begin{align*}
	\mathbb{E}\left[\Vert X^{{(t+1)}} - \Bar{X}^{{(t+1)}} \Vert_F^2 + \Vert X^{{(t+1)}} - \hat{X}^{{(t+2)}} \Vert_F^2 \right] \leq \left( 1-\frac{p}{2} \right)\mathbb{E}\left[ \Vert\Bar{X}^{{(t)}} - X^{{(t)}}\Vert_F^2  + \Vert \hat{X}^{{(t+1)}} - X^{{(t)}} \Vert_F^2 \right] + \frac{2A}{p}\eta_{t}^2
	\end{align*}
	Using $e_t : =  \left[ \Vert\Bar{X}^{{(t)}} - X^{{(t)}}\Vert_F^2  + \Vert \hat{X}^{{(t+1)}} - X^{{(t)}} \Vert_F^2 \right] $, above can be written as:
	\begin{align} \label{suppl_lemm_rec_rel}
	\mathbb{E}[e_{t+1}] \leq \left( 1- \frac{p}{2} \right)\mathbb{E}[e_t] + \frac{2A}{p} \eta_t^2
	\end{align}
	Thus, employing Lemma \ref{suppl_lem_e_seq}, the sequence $\mathbb{E}[e_{t}]$ follows the bound for all $t$: 
	\begin{align*}
	\mathbb{E}[e_t] \leq \frac{20A\eta_{{t}}^2}{p^2}
	\end{align*}
	Note that we also have :  $\mathbb{E}\Vert\Bar{X}^{{(t)}} - X^{{(t)}}\Vert_F^2 \leq \mathbb{E} \left[ \Vert\Bar{X}^{{(t)}} - X^{{(t)}}\Vert_F^2  + \Vert \hat{X}^{{(t+1)}} - X^{{(t)}} \Vert_F^2 \right] := \mathbb{E}[e_{t}] $. Thus, we get:
	\begin{align*}
	\mathbb{E}\Vert\Bar{X}^{{(t)}} - X^{{(t)}}\Vert_F^2 \leq \frac{20A\eta_{{t}}^2}{p^2}
	\end{align*}
	where $A := 2nG^2 + \frac{p}{2} \left( \frac{8nG^2}{\omega} + \frac{5 \omega n c_0}{4} \right) $ and $p = \left( 1 - \frac{\delta^2 \omega}{644} \right)$. 
\end{proof}
%------------Lemma-------
\begin{lemma} \label{suppl_lem_coeff_calc}
	Consider:
	\begin{align*}
	\pi_1 (\gamma) & := \gamma^2 \beta^2 (1+\alpha_1^{-1}) + (1+\gamma \beta )^2 (1+\alpha_4) (1+\alpha_3) (1+\alpha_2) (1-\omega) \\
	\pi_2 (\gamma) & := (1-\delta \gamma)^2(1+\alpha_1) + \gamma^2 \beta^2 (1+\alpha_4^{-1}) (1+\alpha_3) (1+\alpha_2) (1-\omega) \\
	\pi_3 & := (1+\alpha_3^{-1}) (1+\alpha_2) (1-\omega) nG^2 + (1+\alpha_2)\omega n c_0 + (1+\alpha_2^{-1})nG^2 
	\end{align*}
	and the following choice of variables:
	\begin{align*}
	\alpha_1 := \frac{\gamma \delta}{2}, \, 
	\alpha_2 := \frac{\omega}{4}, \,
	\alpha_3 := \frac{\omega}{4}, \,
	\alpha_4 := \frac{\omega}{4} \\
	\gamma^* := \frac{2 \delta \omega}{64 \delta + \delta^2 + 16 \beta^2 + 8 \delta \beta^2 - 16\delta \omega} \\
	\end{align*}
	Then, it can be shown that:
	\begin{align*}
	max \{ \pi_1 (\gamma^*) , \pi_2 (\gamma^*) \} & \leq 1 - \frac{\delta^2 \omega}{644} \hspace{0.5cm}, \hspace{0.5cm}
	\pi_3 \leq \frac{8nG^2}{\omega} + \frac{5\omega nc_0}{4}
	\end{align*}
\end{lemma}
\begin{proof}
	Consider:
	\begin{align*}
	(1+\alpha_4) (1+\alpha_3) (1+\alpha_2) (1-\omega) & = (1+\frac{\omega}{4})^3 (1-\omega) \\
	& = \left( 1 - \frac{\omega^4}{64} - \frac{11 \omega^3}{64} - \frac{9 \omega^2}{16} - \frac{\omega}{4} \right) \\
	& \leq \left( 1 - \frac{\omega}{4} \right)
	\end{align*}
	This gives us:
	\begin{align*}
	\pi_1(\gamma) \leq \gamma^2\beta^2\left(1+\frac{2}{\gamma \delta} \right) + (1+\gamma\beta)^2 \left( 1 - \frac{\omega}{4} \right)
	\end{align*}
	Noting that $\gamma^2 \leq \gamma $ (for $\gamma \leq 1 $ which is true for $\gamma^*$ ) and $\beta \leq 2$, we have:
	\begin{align*}
	\pi_1(\gamma) \leq \beta^2\left(\gamma +\frac{2\gamma}{\delta} \right) + (1+8\gamma) \left( 1 - \frac{\omega}{4} \right)
	\end{align*}
	Substituting value of $\gamma^*$ in above, it can be shown that:
	\begin{align*}
	\pi_1(\gamma^*) \leq 1 - \frac{\delta^2\omega}{4(64 \delta + \delta^2 + 16 \beta^2 + 8 \delta \beta^2 - 16\delta \omega)}
	\end{align*}
	Now we note that:
	\begin{align*}
	\pi_2 (\gamma) & =  (1-\delta \gamma)^2 \left(1+\frac{\delta \gamma}{2} \right) + \gamma^2 \beta^2 \left( 1+\frac{4}{\omega} \right) \left(1+\frac{\omega}{4} \right)^2 (1-\omega) 
	\intertext{where we use the fact that for $x = \delta \gamma \leq 1 $ : $\left( 1 - x  \right) \left(1 + \frac{x}{2}\right) \leq \left( 1 - \frac{x}{2}  \right) $ and $ \left( 1 -x \right) \left( 1 - \frac{x}{2} \right) \leq \left( 1 - \frac{x}{2}\right)^2 $ }
	& \leq \left( 1-\frac{\gamma \delta}{2} \right)^2 + \gamma^2 \beta^2 \left( 1+\frac{4}{\omega} \right) \left(1+\frac{\omega}{4} \right)^2 (1-\omega)\\
%	& = \left( 1-\frac{\gamma \delta}{2} \right)^2 + \gamma^2 \beta^2 \left( 1+\frac{4}{\omega} \right) \left(1+\frac{\omega^2}{16} + \frac{\omega}{2} \right) (1-\omega) \\
	& = \left( 1-\frac{\gamma \delta}{2} \right)^2 + \gamma^2 \beta^2 \left(3+\frac{3\omega}{4}+\frac{\omega^2}{16} + \frac{4}{\omega} \right) (1-\omega) \\
	& \leq \left( 1-\frac{\gamma \delta}{2} \right)^2 + \gamma^2 \beta^2 \frac{4}{\omega} \, : = \zeta(\gamma)
	\end{align*}
	Note that $\zeta(\gamma)$ is convex and quadratic in $\gamma$, the minimum value is attained at $\gamma' = \frac{2 \delta \omega}{16 \beta^2 + \delta^2 \omega}$ with value $\zeta(\gamma') = \frac{16\beta^2}{16\beta^2 + \omega \delta^2}$ \\
	By Jensen's inequality, we note that for any $\lambda \in [0,1]$
	\begin{align*}
	\zeta(\lambda \gamma') \leq (1-\lambda) \zeta(0) + \lambda \zeta(\gamma') = 1 - \lambda \frac{\delta^2 \omega}{16 \beta^2 + \delta^2 \omega}
	\end{align*}
	For the choice $\lambda' = \frac{16\beta^2 + \omega \delta^2}{64 \delta + \delta^2 + 16 \beta^2 + 8 \delta \beta^2 - 16\delta \omega}$, it can be seen that $\lambda' \gamma' = \gamma^*$. Thus we get:
	\begin{align*}
	\pi_2(\gamma^*) \leq  \zeta(\lambda' \gamma')  & \leq 1 - \frac{\delta^2\omega}{(64 \delta + \delta^2 + 16 \beta^2 + 8 \delta \beta^2 - 16\delta \omega)} \\
	& \leq 1 - \frac{\delta^2\omega}{4(64 \delta + \delta^2 + 16 \beta^2 + 8 \delta \beta^2 - 16\delta \omega)}
	\end{align*}
	Now we note the value of $\pi_3$ (here $\omega \in (0,1)$):
	\begin{align*}
	\pi_3 & = \left( 1+\frac{4}{\omega} \right)nG^2 + \left( 1 + \frac{\omega}{4} \right) (1 - \omega)\left( 1+\frac{4}{\omega} \right) nG^2 + \left( 1+\frac{\omega}{4} \right)\omega n c_0\\
	& = \left( 1+\frac{4}{\omega} \right) nG^2 \left[ 2 - \frac{3\omega}{4} - \frac{\omega^2}{4} \right] + \left( 1+\frac{\omega}{4} \right)\omega n c_0\\
	& \leq 2nG^2\left( 1+\frac{4}{\omega} \right)\left( 1-\frac{3\omega}{8} \right)+ \frac{5\omega n c_0}{4} = 2nG^2\left( 1-\frac{3\omega}{8} + \frac{4}{\omega} - \frac{3}{2} \right) + \frac{5\omega n c_0}{4} \\
	& \leq \frac{8nG^2}{\omega} + \frac{5\omega n c_0}{4}
	\end{align*}
	Thus we have:
	\begin{align*}
	max \{ \pi_1 (\gamma^*) , \pi_2 (\gamma^*) \} & \leq 1 - \frac{\delta^2\omega}{4(64 \delta + \delta^2 + 16 \beta^2 + 8 \delta \beta^2 - 16\delta \omega)}
	\intertext{Using crude estimates $\delta \leq 1, \omega \geq 0, \beta \leq2, $}
	& \leq 1 - \frac{\delta^2 \omega}{644}
	\end{align*}
\end{proof}
%------------Lemma-------
\begin{lemma} \label{suppl_lem_e_seq}
	Consider the sequence \{$e_{t}$\} given by
	\begin{align*}
	e_{{t+1}} \leq \left( 1-\frac{p}{2} \right)e_{t} + \frac{2}{p}\eta_{t}^2A
	\end{align*}
	For a parameter $p >0$, stepsize $\eta_t = \frac{b}{t+a}$, for parameter $a \geq \frac{5}{p}$ and arbitrary $b >0$, we have:
	\begin{align*}
	e_{t} \leq \frac{20}{p^2}A\eta_{{t}}^2
	\end{align*}
\end{lemma}
\begin{proof}
	We will proceed the proof by induction. Note that for t=0, $e_{0}:=0$, thus statement is true. Assume the statement holds for index $t$, then for index $(t+1)$:  
	\begin{align*}
	e_{{t+1}} \leq \left( 1- \frac{p}{2} \right)e_{{t}} + \frac{2}{p}A\eta_{{t}}^2 \leq  \left( 1- \frac{p}{2} \right)\frac{20}{p^2}A\eta_{{t}}^2 + \frac{2}{p}A\eta_{{t}}^2  = \frac{A\eta_{{t}}^2}{p^2}(20-8p) \stackrel{(p \geq \frac{5}{a})}{\leq} \frac{20A\eta_{{t}}^2}{p^2}\left( 1- \frac{2}{a} \right)  
	\end{align*}
	Now, we note the following:
	\begin{align*}
	(a+ {t+1})^2 \left( 1- \frac{2}{a} \right)     & = (a+ 1)^2 + 2(a+ {t}) + 1 - \left[ \frac{2(a+ {t})^2}{a} + \frac{4(a+ {t})}{a} + \frac{2}{a} \right] \\
	& \leq (a+ {t})^2 + 2(a+ {t}) + 1 - \left[ 2(a+ {t}) + 4 \right] \\
	& \leq (a+ {t})^2
	\end{align*}
	Thus, for $\eta_{{t+1}} = \frac{b}{a + {t+1} }$, we get:
	\begin{align*}
	\eta_{{t}}^2 \left( 1- \frac{2}{a} \right) \leq \eta_{{t+1}}^2
	\end{align*}
	Substituting the above bound in the bound for $e_{t+1}$ gives us:
	\begin{align*}
	e_{{t+1}} \leq \frac{20A\eta_{{t+1}}^2}{p^2}
	\end{align*}
	Thus, by induction : $e_{{t}} \leq \frac{20A\eta_{{t}}^2}{p^2}$ for all $t$.
\end{proof}
%------------------------------------------------------------------
%------------------------------------------------------------------
\subsection{Proof of Theorem \ref{thm_cvx} (Strongly convex objective)} \label{proof_thm_cvx}
\begin{proof}[Proof of Theorem ~\ref{thm_cvx}]
	From Lemma \ref{suppl_cvx_lemm}, we have that :
	\begin{align*}
	\mathbb{E}_{\xi_t} \Vert \Bar{x}^{(t+1)} - x^* \Vert^2 \leq \left( 1-\frac{\eta_t \mu}{2} \right) \Vert \Bar{x}^{(t)} - x^* \Vert^2 + \frac{\eta_t^2 \Bar{\sigma}^2}{n} - 2\eta_t (1-2L\eta_t) (f(\Bar{x}^{(t)}) - f^*) + 
	\eta_t \left(  \frac{2\eta_t L^2 + L + \mu}{n}  \right) \sum_{j=1}^n \Vert \Bar{x}^{(t)} - x_j^{(t)} \Vert^2
	\end{align*}
	Taking expecatin w.r.t the whole process gives us:
	\begin{align} \label{suppl_cvx_lemm_use}
	\mathbb{E}\Vert \Bar{x}^{(t+1)} - x^* \Vert^2 \leq \left( 1-\frac{\eta_t \mu}{2} \right) \mathbb{E} \Vert \Bar{x}^{(t)} - x^* \Vert^2 + \frac{\eta_t^2 \Bar{\sigma}^2}{n} - 2\eta_t (1-2L\eta_t) (\mathbb{E}f(\Bar{x}^{(t)}) - f^*) + 
	\eta_t \left(  \frac{2\eta_t L^2 + L + \mu}{n}  \right) \sum_{j=1}^n \mathbb{E}\Vert \Bar{x}^{(t)} - x_j^{(t)} \Vert^2
	\end{align}
	The last term in (\ref{suppl_cvx_lemm_use}), can be bounded by using Lemma \ref{lem_dec_sgd} which gives us:
	%\begin{align}
	%\Gamma_{t} = \sum_{j=1}^n \mathbb{E}\Vert \Bar{x}^{(t)} - x_j^{(t)} \Vert^2 = \mathbb{E} \Vert X^{(t)} - \Bar{X}^{(t)} \Vert_F^2
	%\end{align}
	%Using Lemma0.7, for $A= 2nG^2 + \frac{p}{2}\left( \frac{8nG^2}{\omega} + \frac{5\omega n c_0}{4} \right)$
	%\begin{align}
	%\Gamma_{t} \leq \frac{20A}{p^2} \eta_t^2
	%\end{align}
	%Substituting (92) in (90) (Lemma0.10) yields:
	\begin{align*}
	\mathbb{E} \Vert \Bar{x}^{(t+1)} - x^* \Vert^2 & \leq \left( 1-\frac{\eta_t \mu}{2} \right) \mathbb{E} \Vert \Bar{x}^{(t)} - x^* \Vert^2 + \frac{\eta_t^2 \Bar{\sigma}^2}{n} - 2\eta_t (1-2L\eta_t) (\mathbb{E}f(\Bar{x}^{(t)}) - f^*)  + \eta_t \left(  \frac{2\eta_t L^2 + L + \mu}{n}  \right)\frac{20A}{p^2}\eta_t^2 
	\intertext{where $A= 2nG^2 + \frac{p}{2}\left( \frac{8nG^2}{\omega} + \frac{5\omega n c_0}{4} \right)$}
	& \stackrel{(b)}{\leq} \left( 1-\frac{\eta_t \mu}{2} \right) \mathbb{E} \Vert \Bar{x}^{(t)} - x^* \Vert^2 - \eta_t (\mathbb{E}f(\Bar{x}^{(t)}) - f^*) + \frac{\eta_t^2 \Bar{\sigma}^2}{n}  + \eta_t^3 \left(  \frac{2L + \mu}{n}  \right) \frac{20A}{p^2}
	\end{align*}
	where in $(b)$, we use $a \geq \text{max} \{ \frac{16L}{\mu}, \frac{5}{p}\} $ implying $\eta_t \leq \frac{1}{4L}$ which gives $2L\eta_t - 1 \leq -\frac{1}{2}$ and $(2\eta_t L^2 + L + \mu) \leq (2L + \mu)$ for $\eta_t := \frac{4}{\mu (a+t)}$ \\ 
	%For $\eta_t = \frac{4}{\mu (a+t)}$ and $a \geq \text{max} \{ \frac{16L}{\mu}, \frac{5}{p}\} $, we have $\eta_t \leq \frac{1}{4L}$. This gives:
	%\begin{align*}
	%2L\eta_t - 1 \leq -\frac{1}{2} \\
	%(2\eta_t L^2 + L + \mu) \leq (2L + \mu)
	%\end{align*}
	%Using (95) and (96) in (93-94), we have:
	%\begin{align}
	%\mathbb{E} \Vert \Bar{x}^{(t+1)} - x^* \Vert^2 & \leq \left( 1-\frac{\eta_t \mu}{2} \right) \mathbb{E} \Vert \Bar{x}^{(t)} - x^* \Vert^2 - \eta_t (f(\Bar{x}^{(t)}) - f^*) + \frac{\eta_t^2 \Bar{\sigma}^2}{n}  \\ 
	%& \hspace{1cm} + \eta_t^3 \left(  \frac{2L + \mu}{n}  \right) \frac{20A}{p^2}
	%\end{align}
	Substituting $A = 2nG^2 + \frac{p}{2}\left( \frac{8nG^2}{\omega} + \frac{5\omega n c_0}{4} \right)$ yields:
	\begin{align*}
	\mathbb{E} \Vert \Bar{x}^{(t+1)} - x^* \Vert^2 & \leq \left( 1-\frac{\eta_t \mu}{2} \right) \mathbb{E} \Vert \Bar{x}^{(t)} - x^* \Vert^2 - \eta_t (\mathbb{E}f(\Bar{x}^{(t)}) - f^*) + \frac{\eta_t^2 \Bar{\sigma}^2}{n} + \eta_t^3 \left(  \frac{2L + \mu}{n}  \right) \frac{20}{p^2}\left( 2nG^2 + \frac{p}{2}\left( \frac{8nG^2}{\omega} + \frac{5\omega n c_0}{4} \right) \right)
	\end{align*}
	We use Lemma \ref{suppl_cvx_lemma_stitch} for the sequence relation above by defining:
	\begin{align*}
	a_t & = \mathbb{E} \Vert \Bar{x}^{(t)} - x^* \Vert^2 \\
	e_t & = \mathbb{E}f(\Bar{x}^{(t)}) - f^* \\
	P & = 1 \\ 
	Q & = \frac{ \Bar{\sigma}^2}{n} \\
	R & = \left(  \frac{2L + \mu}{n}  \right) \frac{20}{p^2}\left( 2nG^2 + \frac{p}{2}\left( \frac{8nG^2}{\omega} + \frac{5\omega n c_0}{4} \right) \right)
	\end{align*}
	%Thus we get:
	%\begin{align*}
	%\frac{1}{S_T} \sum_{t=0}^{T-1}w_t e_t \leq \frac{\mu a^3}{8S_T}\Vert \bar{x}^{(0)} - x^* \Vert^2 + \frac{2T(T+2a)}{\mu S_T}\frac{ \Bar{\sigma}^2}{n} + \frac{16T}{\mu^2 S_T}\left(  \frac{2L + \mu}{n}  \right) \frac{20}{p^2}\left( 2nG^2 + \frac{pc_1}{2} \right)
	%\end{align*}
	%Substituting value of $c_1 = \frac{8nG^2}{\omega} + \frac{5\omega n c_0}{4}$ gives:
	For $w_t = (a+t)^2$, $a_0 =  \Vert \Bar{x}^{(0)} - x^* \Vert^2 $ and $e_t = \mathbb{E}f(\Bar{x}^{(t)}) - f^*$, this gives us the relation:
	\begin{align*}
	\frac{1}{S_T} \sum_{t=0}^{T-1}w_t e_t \leq \frac{\mu a^3}{8S_T}a_0 + \frac{2T(T+2a)}{\mu S_T}\frac{ \Bar{\sigma}^2}{n} + \frac{16T}{\mu^2 S_T}\left(  \frac{2L + \mu}{n}  \right) \frac{20}{p^2}\left( 2nG^2 + \frac{p}{2}\left(\frac{8nG^2}{\omega} + \frac{5\omega n c_0}{4} \right) \right)
	\end{align*}
	From the convexity of $f$, we have finally have: 
	\begin{align*}
	\mathbb{E}f(x_{avg}^{(T)}) - f^* \leq \frac{\mu a^3}{8S_T}a_0 + \frac{2T(T+2a)}{\mu S_T}\frac{ \Bar{\sigma}^2}{n} + \frac{16T}{\mu^2 S_T}\left(  \frac{2L + \mu}{n}  \right) \frac{20}{p^2}\left( 2nG^2 + \frac{p}{2}\left(\frac{8nG^2}{\omega} + \frac{5\omega n c_0}{4} \right) \right)
	\end{align*}
	%(where $e_t = f(\Bar{x}^{(t)}) - f^*$)
	where  $\Bar{x}^{(T)}_{avg} = \frac{1}{S_T} \sum_{t=0}^{T-1}w_t \bar{x}^{(t)}$.
	This completes the proof of Theorem \ref{thm_cvx}.
\end{proof}
%------------Lemma-------
\begin{lemma} \label{suppl_cvx_lemma_stitch}
	(From \cite{stich_sparsified_2018})
	Let $\{ a_t \}_{t \geq 0}, a_t \geq 0, e_t \}_{t \geq 0}, e_t \geq 0 $ be sequences satisfying :
	\begin{align*}
	a_{t+1} \leq (1-\mu \eta_t) a_{t} - \eta_t e_t P + \eta_t^2Q + \eta_t^3R,
	\end{align*}
	for stepsizes $\eta_t = \frac{4}{\mu (a+t)} $ and constants $P>0,Q,R \geq 0, \mu>0, a>1. $ Then :
	\begin{align*}
	\frac{P}{S_T} \sum_{t=0}^{T-1}w_t e_t \leq \frac{\mu a^3}{4S_T}a_0 + \frac{2T(T+2a)}{\mu S_T}Q + \frac{16T}{\mu^2 S_T}R,
	\end{align*}
	for $w_t = (a+t)^2$ and $S_T := \sum_{t=0}^{T-1}w_t = \frac{T}{6} (2T^2+6aT-3T+6a^2-6a+1) \geq \frac{1}{3}T^3$
\end{lemma}
%--------------------------------------------------------------------
%--------------------------------------------------------------------
\subsection{Proof of Theorem \ref{thm_noncvx_var} (Non-convex objective with varying step size)} \label{proof_thm_noncvx_var}
\begin{proof}[Proof of Theorem~\ref{thm_noncvx_var}:]
	We now take expectation w.r.t the whole process and use Lemma \ref{lem_dec_sgd} to bound  $\sum_{j=1}^n \Vert \bar{x}_{t} - x_t^{(j)} \Vert^2$ :  
	\begin{align*}
	\mathbb{E} f(\bar{x}_{t+1}) & \leq \mathbb{E} f(\bar{x}_{t}) - \eta_t \left( \frac{1}{2} - 2L\eta_t \right) \mathbb{E} \Vert \nabla f(\bar{x}_{t})  \Vert_2^2 + \left( \frac{\eta_tL}{2n} + \frac{2L^2\eta_t^2}{n} \right) \frac{20\eta_t^2A}{p^2} + L\eta_t^2 \bar{\sigma}^2 
	\intertext{where $A= 2nG^2 + \frac{p}{2}\left( \frac{8nG^2}{\omega} + \frac{5\omega n c_0}{4} \right)$ . For the choice of $\eta_t = \frac{b}{(t+a)}$ and $a \geq \text{max} \left\{  \frac{5}{p}, 8bL  \right\}  $, we have $\eta_t \leq \frac{1}{8L}$: }
	& \leq \mathbb{E} f(\bar{x}_{t}) - \frac{\eta_t}{4} \mathbb{E} \Vert \nabla f(\bar{x}_{t})  \Vert_2^2 +  \frac{10LA}{np^2}\eta_t^3 + \frac{40L^2A}{np^2}\eta_t^4 + \frac{L\eta_t^2 \bar{\sigma}^2}{n}
	\end{align*}
	Rearranging the terms and summing from $0$ to $T-1$, we get:
	\begin{align} \label{non_cvx_rec_rel}
	\sum_{t=0}^{T-1} \eta_t  \mathbb{E} \Vert \nabla f(\bar{x}_{t}) \Vert_2^2  \leq 4 \left( f(\bar{x}_{0}) - \mathbb{E} f(\bar{x}_{T}) \right) +  \frac{40LA}{np^2} { \sum_{t=0}^{T-1}\eta_t^3} + \frac{160L^2A}{np^2}{ \sum_{t=0}^{T-1}\eta_t^4} + \frac{4L \bar{\sigma}^2}{n} {\sum_{t=0}^{T-1}\eta_t^2} \notag
	\intertext{Dividing both sides by $\sum_{t=0}^{T-1}\eta_t$ , we have:}
	\frac{\sum_{t=0}^{T-1} \eta_t  \mathbb{E} \Vert \nabla f(\bar{x}_{t}) \Vert_2^2}{{\sum_{t=0}^{T-1}\eta_t}}  \leq \frac{4 \left( f(\bar{x}_{0}) - \mathbb{E} f(\bar{x}_{T-1}) \right) }{\sum_{t=0}^{T-1}\eta_t} +  \frac{40LA}{np^2} \frac{ \sum_{t=0}^{T-1}\eta_t^3}{\sum_{t=0}^{T-1}\eta_t} + \frac{160L^2A}{np^2}\frac{ \sum_{t=0}^{T-1}\eta_t^4}{\sum_{t=0}^{T-1}\eta_t} + \frac{4L \bar{\sigma}^2}{n} \frac{\sum_{t=0}^{T-1}\eta_t^2}{\sum_{t=0}^{T-1}\eta_t}
	\end{align}
	We now note the following bounds on the sum of series $\eta_t = \frac{b}{t+a}$ :
	\begin{align*} 
	\sum_{t=0}^{T-1} \eta_t \geq \int_{0}^{T-1} \frac{b}{t+a} dt = b \log \left( \frac{T+a-1}{a} \right) \\
	\sum_{t=0}^{T-1} \eta_t^2 \leq \eta_0^2 + \int_{0}^{T-1} \frac{b^2}{(t+a)^2} dt  \leq \eta_0^2 + \int_{0}^{\inf} \frac{b^2}{(t+a)^2} dt = \eta_0^2 + \frac{b^2}{a} = \frac{b^2}{a^2} + \frac{b^2}{a}  \\
	\sum_{t=0}^{T-1} \eta_t^3 \leq \eta_0^3 + \int_{0}^{T-1} \frac{b^3}{(t+a)^3} dt  \leq \eta_0^3 + \int_{0}^{\inf} \frac{b^3}{(t+a)^3} dt = \eta_0^3 + \frac{b^3}{2a^2} = \frac{b^3}{a^3} + \frac{b^3}{2a^2} \\
	\sum_{t=0}^{T-1} \eta_t^4 \leq \eta_0^4 + \int_{0}^{T-1} \frac{b^4}{(t+a)^4} dt  \leq \eta_0^4 + \int_{0}^{\inf} \frac{b^4}{(t+a)^4} dt = \eta_0^3 + \frac{b^4}{3a^3} = \frac{b^4}{a^4} + \frac{b^4}{3a^3}
	\end{align*}
	Substituting these bounds in (\ref{non_cvx_rec_rel}) and noting that $\mathbb{E} f(\bar{x}_T) \geq f(x^*) = f^*  $   we get:
	\begin{align*}
	\frac{\sum_{t=0}^{T-1} \eta_t  \mathbb{E} \Vert \nabla f(\bar{x}_{t}) \Vert_2^2}{{\sum_{t=0}^{T-1}\eta_t}}  \leq \frac{4 \left( f(\bar{x}_{0}) - f^* \right) }{b \log \left( \frac{T+a-1}{a} \right)} +  \frac{40LA}{np^2} \frac{\left(\frac{b^3}{a^3} + \frac{b^3}{2a^2}\right)}{b \log \left( \frac{T+a-1}{a} \right)} + \frac{160L^2A}{np^2}\frac{ \left(\frac{b^4}{a^4} + \frac{b^4}{3a^3} \right)}{b \log \left( \frac{T+a-1}{a} \right)} + \frac{4L \bar{\sigma}^2}{n} \frac{\left(\frac{b^2}{a^2} + \frac{b^2}{a}\right)}{b \log \left( \frac{T+a-1}{a} \right)}
	\end{align*}
	where $A= 2nG^2 + \frac{p}{2}\left( \frac{8nG^2}{\omega} + \frac{5\omega n c_0}{4} \right)$. This completes proof of Theorem \ref{thm_noncvx_var} .
\end{proof} 
%--------------------------------------------------------------------
%--------------------------------------------------------------------
\subsection{Proof of Lemma \ref{lemm_dec_sgd_fix}} \label{proof_lemm_dec_sgd_fix}
\begin{lemma*} (Restating Lemma \ref{lemm_dec_sgd_fix} )
	Consider the sequence of updates as in Algorithm \ref{alg_dec_sgd} with some constant step size $\eta$. Then in matrix notation from Appendix \ref{mat_not_sec}, we have:
	\begin{align*}
	\mathbb{E}\sum_{j=1}^n \Vert \bar{x}_{t} - x_t^{(j)} \Vert^2 = \mathbb{E}\Vert\Bar{X}^{{(t)}} - X^{{(t)}}\Vert_F^2 \leq \frac{4A\eta^2}{p^2}
	\end{align*}
	where  $p = \frac{\delta^2 \omega}{644} $, $\delta := 1 - | \lambda_2(W)|$, $\omega$ is contraction parameter for quantization operator $Q$, $ A=2nG^2 + \frac{p}{2} \left( \frac{8nG^2}{\omega} + \frac{5\omega n c_0}{4} \right) $
\end{lemma*}
\begin{proof}[Proof of Lemma \ref{lemm_dec_sgd_fix}]
	We use the same steps for the Proof of Lemma \ref{lem_dec_sgd} wtih $\eta_t = \eta$, till eqn (\ref{suppl_lemm_rec_rel}). This gives us:
	\begin{align*} 
	\mathbb{E}[e_{t+1}] \leq \left( 1- \frac{p}{2} \right)\mathbb{E}[e_t] + \frac{2A}{p} \eta^2
	\end{align*}
	where   $e_{t+1} := \Vert X^{(t+1)} - \Bar{X}^{(t+1)} \Vert_F^2 + \Vert X^{(t+1)} - \hat{X}^{(t+2)} \Vert_F^2$ and  $A := 2nG^2 + \frac{p }{2}\left( \frac{8nG^2}{\omega} + \frac{5\omega n c_0}{4} \right) $. \\
	It can be seen that $\mathbb{E}[e_t] \leq \frac{4A}{p^2}\eta^2$ satisfies the recursion above. Using $\mathbb{E}[ \Vert X^{(t)} - \Bar{X}^{(t)} \Vert_F^2 ] \leq \mathbb{E}[e_t] $ completes the proof.
\end{proof}
%--------------------------------------------------------------------
%--------------------------------------------------------------------
\subsection{Proof of Theorem \ref{thm_noncvx_fix} (Non-convex objective with constant step size)} \label{proof_thm_noncvx_fix}
\begin{proof}[Proof of Theorem~\ref{thm_noncvx_fix}:]
The proof follows the same steps as Proof of Theorem \ref{thm_noncvx_var} till (\ref{non_cvx_eqn_temp}) with $\eta_t = \eta = \sqrt{\frac{n}{T}}$
\begin{align}
	\mathbb{E} _{\xi_t} [f(\bar{x}_{t+1})] 	& \leq  f(\bar{x}_{t}) - \eta \left( \frac{1}{2} - 2L\eta \right)  \Vert \nabla f(\bar{x}_{t})  \Vert_2^2 + \left( \frac{\eta L}{2n} + \frac{2L^2\eta^2}{n} \right) \sum_{j=1}^n  \Vert \bar{x}_{t} - x_t^{(j)} \Vert^2 + \frac{L\eta^2 \bar{\sigma}^2}{n} 
\end{align}
where $\xi_t$ denotes stochastic samples at timestep $t$. Taking expectation w.r.t the entire process and using Lemma \ref{lemm_dec_sgd_fix}:
%We use a modified version of Lemma 0.9. Specifically:
%\begin{align}
%e_{t+1} \leq \left( 1 - \frac{p}{2} \right) e_t + \frac{2A}{p} \eta^2
%\end{align}
%It can be easily seen that $e_t \leq \frac{4A}{p^2}\eta^2$ satisfies the recursion and thus the difference is in bounding the term $\Gamma_t = \Vert X^{(t)} - \bar{X}^{(t)} \Vert_F^2 $ as $\Gamma_t \leq \frac{4A}{p^2}\eta^2 $. \\
%Thus the proof proceeds as:
\begin{align*}
\mathbb{E} f(\bar{x}_{t+1}) & \leq \mathbb{E} f(\bar{x}_{t}) - \eta \left( \frac{1}{2} - 2L\eta \right) \mathbb{E} \Vert \nabla f(\bar{x}_{t})  \Vert_2^2 + \left( \frac{\eta L}{2n} + \frac{2L^2\eta^2}{n} \right) \frac{4\eta^2A}{p^2} + \frac{L\bar{\sigma}^2\eta^2}{n}
\intertext{where $A := 2nG^2 + \frac{p }{2}\left( \frac{8nG^2}{\omega} + \frac{5\omega n c_0}{4} \right) $ . For the choice of $\eta = \sqrt{\frac{n}{T}}$ and $T \geq 64nL^2$, we have $\eta \leq \frac{1}{8L}$, which gives:}
& \leq \mathbb{E} f(\bar{x}_{t}) - \frac{\eta}{4} \mathbb{E} \Vert \nabla f(\bar{x}_{t})  \Vert_2^2 +  \frac{2LA}{np^2}\eta^3 + \frac{8L^2A}{np^2}\eta^4 + \frac{L\bar{\sigma}^2\eta^2}{n} 
\end{align*}
Rearranging the terms and summing from $0$ to $T-1$, we get:
\begin{align*}
\sum_{t=0}^{T-1} \eta  \mathbb{E} \Vert \nabla f(\bar{x}_{t}) \Vert_2^2  \leq 4 \left( f(\bar{x}_{0}) - \mathbb{E} f(\bar{x}_{T}) \right) +  \frac{8LA}{np^2} { \sum_{t=0}^{T-1}\eta^3} + \frac{32L^2A}{np^2}{ \sum_{t=0}^{T-1}\eta^4} + \frac{4L\bar{\sigma}^2}{n} {\sum_{t=0}^{T-1}\eta^2}
\end{align*}
Dividing both sides by $\sum_{t=0}^{T-1}\eta$, we finally have:
\begin{align}
%\frac{\sum_{t=0}^{T-1} \eta  \mathbb{E} \Vert \nabla f(\bar{x}_{t}) \Vert_2^2}{{\sum_{t=0}^{T-1}\eta}}  
%& \leq \frac{4 \left( f(\bar{x}_{0}) - \mathbb{E} f(\bar{x}_{T-1}) \right) }{\sum_{t=0}^{T-1}\eta} +  \frac{8LA}{np^2} \frac{ \sum_{t=0}^{T-1}\eta^3}{\sum_{t=0}^{T-1}\eta} + \frac{32L^2A}{np^2}\frac{ \sum_{t=0}^{T-1}\eta^4}{\sum_{t=0}^{T-1}\eta} + \frac{4L\bar{\sigma}^2}{n} \frac{\sum_{t=0}^{T-1}\eta^2}{\sum_{t=0}^{T-1}\eta} \\
%\end{align}
%\begin{align}
%\frac{\sum_{t=0}^{T-1}  \mathbb{E} \Vert \nabla f(\bar{x}_{t}) \Vert_2^2}{T}
\frac{\sum_{t=0}^{T-1}  \mathbb{E} \Vert \nabla f(\bar{x}_{t}) \Vert_2^2}{T}  \leq \frac{4 \left( f(\bar{x}_{0}) - f^*) \right) }{\eta T} +  \frac{8LA}{np^2} \eta^2 + \frac{32L^2A}{np^2}\eta^3 + \frac{4L\bar{\sigma}^2}{n} \eta
\end{align}
where $A= 2nG^2 + \frac{p }{2}\left( \frac{8nG^2}{\omega} + \frac{5\omega n c_0}{4} \right)$. Substituting $\eta = \sqrt{\frac{n}{T}}$ completes the proof.
\end{proof}
