# Supplementary material for: SPARQ-SGD: Event-Triggered and Compressed Communication in Decentralized Stochastic Optimization
Source: arXiv:1910.14280 source file (2020-02-24)
Supplement: Supplementary file 2 [file appendix.tex]

\documentclass{article}
\usepackage[utf8]{inputenc}
\usepackage{amsmath}
\usepackage{amsthm}
\usepackage{amsfonts}
\usepackage{bbm}
\usepackage{algorithm}
\usepackage{algorithmic}
\usepackage{amsmath}
\usepackage{graphicx}
\usepackage{float}
\usepackage{fullpage}
\usepackage[utf8]{inputenc}
\usepackage[english]{babel}
\usepackage{geometry}
\usepackage{appendix}
\usepackage{authblk}
\usepackage{nicefrac}
\geometry{
	a4paper,
	total={170mm,257mm},
	left=10mm,
	right=10mm,
	top=20mm,
	% textwidth = 10cm,
}
\newtheorem*{theorem*}{Theorem}

\newtheorem*{lemma*}{Lemma}

\begin{document}
	\input{remarks.tex}	
	\input{suppl_dec_sgd_li.tex}
\end{document}
